# Supplementary material for: Regime-Adaptive Bayesian Optimization via Dirichlet Process Mixtures of Gaussian Processes
Source: arXiv:2601.20043 source file (2026-07-28)
Supplement: Supplementary file 1 [file suppl_proof-sketch.tex]

\newpage

\section{***DRAFT OUTLINE*** Proof of regret bound and convergence}
Our theoretical result shows that the convergence of ordinary GP-EI is conditionally inherited by RAMBO.
The proof follows a two-part strategy. First, we use a well-known result from the literature and show that it directly applies cluster-wise, i.e. based on the cluster marginal likelihood. In a second step, we infer the mixture regret bound and convergence through cluster-wise conditioning on the DP.
%
%
%\subsection{Tran The path}
%
\subsection{Expected Improvement}

We start with Theorem 1 in \cite{tran-the2022}, which provides convergence guarantees for EI with a modified exploration parameter. This modification  is crucial for the proof to hold for noisy BO. For noise-less BO, this part of the proof simplifies significantly and we can instead use  \emph{ordinary} EI based on results by \cite{bull2011convergence}. However, our novelty is the synthesis of the known strategies for GPs with a cluster-wise DP argument, rather than a specific setting and corresponding strategy for a single GP alone. As such, the settings and strategies are exchangeable and we limit ourselves do demonstrating it for noisy BO with modified EI. 
 
Let
\[
x^\star \in \arg\max_{x\in\mathcal X} f(x)
\]
denote a global maximizer of the unknown function $f$.
The cumulative regret after $T$ iterations is defined as
\begin{equation} \label{eq:def-cumulative-regret}
R_T
\;:=\;
\sum_{t=1}^T \bigl( f(x^\star) - f(x_t) \bigr).
\end{equation}
Now consider the following modified EI acquisition function,
\begin{equation} \label{eq:modified-EI}
\alpha_{t,\Omega}^{\mathrm{EI}}(x)
=
\bigl(\mu_{t-1}(x)-\mu_t^+\bigr)
\Phi\!\left(
\frac{\mu_{t-1}(x)-\mu_t^+}{\Omega_t\,\sigma_{t-1}(x)}
\right)
+
\Omega_t\,\sigma_{t-1}(x)\,
\phi\!\left(
\frac{\mu_{t-1}(x)-\mu_t^+}{\Omega_t\,\sigma_{t-1}(x)}
\right),
\end{equation}
with $\Omega_t = \sqrt{\gamma_{t-1} + 1 + \ln\!\left(\tfrac{1}{\delta}\right)}$, wherein $\gamma_t := \max_{A \subset \mathcal X,\ |A| = t} I\!\left( y_A ; f_A \right)$ is the maximum information gain at time $t$. 
%where $\Omega_t =1 \forall t$ restores ordinary EI.

Then Theorem 1 in \cite{tran-the2022} is
\begin{theorem}
    Let $\delta \in (0,1)$. Then with probability at least $1-\delta$, the cumulative regret \eqref{eq:def-cumulative-regret} for the EI acquisition function $\alpha_{t,\Omega}^{\mathrm{EI}}(x)$ \eqref{eq:modified-EI} is bounded as
    \begin{equation}
        R_T = \mathcal{O}(\gamma_T \sqrt{T})
    \end{equation}
\end{theorem}
Since the gating weights $w_k(\mathbf{x}_*) \approx p(z_* = k \mid \mathbf{x}_*, \mathcal{D})$ with regime weights \eqref{eq:regime_weights} $	w_k(\mathbf{x}_*) \propto \frac{n_k}{n + \alpha} \cdot \exp\left(-\frac{1}{2}\log \sigma^2_{*,k}(\mathbf{x}_*)\right)$.
Now introduce the conditional EI as $\mathbb{E}[\max(0, f(x)-f^+) \mid z_\ast =k ] = \alpha_{k, t,\Omega}^{\mathrm{EI}}(x)$. In other words, the mixture EI conditioned on the assignment $z$ is merely the ordinary EI with the single GP (cluster) $k$ that is being conditioned on.
We can condition Theorem D.1. on the regime, i.e. for the conditional EI we restore
\begin{align}
    P\big((R_T \leq \mathcal{O}(\gamma_T \sqrt{T}) \mid z_\ast =k\big) \geq 1-\delta
\end{align}
Then 
\begin{align}
    P\big((R_T \leq \mathcal{O}(\gamma_T \sqrt{T})) &= \sum_k P\big((R_T \leq \mathcal{O}(\gamma_T \sqrt{T}) \mid z_\ast =k\big)\cdot \frac{n_k}{n + \alpha} \exp\left(-\frac{1}{2}\log \sigma^2_{*,k}(\mathbf{x}_*)\right) \\
    % &\leq (1-\delta) K \max_k \frac{n_k}{n + \alpha} \exp\left(-\frac{1}{2}\log \sigma^2_{*,k}(\mathbf{x}_*)\right) \\
    % &\leq (1-\delta) K (n+\alpha)   \max_k  \exp\left(-\frac{1}{2}\log \sigma^2_{*,k}(\mathbf{x}_*)\right) 
    &\geq (1-\delta) \sum_k \frac{n_k}{n + \alpha} \exp\left(-\frac{1}{2}\log \sigma^2_{*,k}(\mathbf{x}_*)\right)\\ 
    &\geq  \frac{1-\delta}{n + \alpha}\sum_k \exp\left(-\frac{1}{2}\log \sigma^2_{*,k}(\mathbf{x}_*)\right)\\ 
\end{align}
since $n_k \geq 1$.

Now consider the modified conditional DPMM-GP-EI
\begin{align}
\text{EI}^{(\Omega)}_{\text{DPMM}}(\mathbf{x}) &= \sum_{k=1}^{K} w_k(\mathbf{x}) \;  \alpha_{t,k}^{\mathrm{EI}}(x) \\
&\leq K\cdot \max_k \big( w_k(\mathbf{x}) \; \alpha_{t,k}^{\mathrm{EI}}(x) \big)
\end{align}

\subsubsection{Auxiliary reminders}

The Cluster Marginal Likelihood \eqref{prop:marginal} is $p(\mathbf{y}_k \mid \mathbf{X}_k, \theta_k) = \mathcal{N}(\mathbf{y}_k \mid \mathbf{0}, \mathbf{K}_k + \sigma^2_{n,k}\mathbf{I})$.

\begin{equation}
\text{EI}_{\text{DPMM}}(\mathbf{x}) = \sum_{k=1}^{K} w_k(\mathbf{x}) \cdot \sigma_{*,k}(\mathbf{x}) [\gamma_k \Phi(\gamma_k) + \phi(\gamma_k)]
\end{equation}

 \begin{theorem}[Cumulative Regret Bound]
Let $f \sim \mathcal{GP}(0, k)$ with $\|f\|_k \leq B$. Using DPMM-GP-UCB with $\beta_t = 2B^2 + 300\gamma_t\log^3(t/\delta)$:
\begin{equation}
R_T = \sum_{t=1}^T (f(\mathbf{x}^*) - f(\mathbf{x}_t)) = O(\sqrt{T\gamma_T \log T})
\end{equation}
with probability at least $1-\delta$, where $\gamma_T$ is the maximum information gain.
\end{theorem}

%%%%%%%%%

\subsubsection{Bull path}
\begin{theorem}[Bull, 2011 --- Convergence rate of Expected Improvement]
Let $\mathcal X \subset \mathbb{R}^d$ be compact with non-empty interior, and let
$\pi$ be a Gaussian process prior with covariance kernel $K_\theta$.
Denote by $\mathcal H_\theta(\mathcal X)$ the associated reproducing-kernel Hilbert space.

For a strategy $u$, define the simple regret after $n$ evaluations by
\[
L_n(u,\mathcal H_\theta(\mathcal X),R)
:=
\sup_{\|f\|_{\mathcal H_\theta(\mathcal X)} \le R}
\mathbb E_f\!\left[f(x_n^\star)-\min_{x\in\mathcal X} f(x)\right],
\]
where $x_n^\star$ is the best point observed up to time $n$.
Assume the kernel $K_\theta$ satisfies Assumptions~1--4 of \cite{Bull2011},
with smoothness parameter $\nu>0$ and logarithmic exponent $\alpha \ge 0$.
Then the Expected Improvement strategy with fixed prior $\pi$ satisfies
\[
L_n(\mathrm{EI}(\pi),\mathcal H_\theta(\mathcal X),R)
=
\begin{cases}
O\!\left(n^{-\nu/d}(\log n)^{\alpha}\right), & \nu \le 1,\\[6pt]
O\!\left(n^{-1/d}\right), & \nu > 1.
\end{cases}
\]
\end{theorem}

\subsection{Upper confidence bound}

\subsubsection{Simple GP}

\newcommand{\cX}{\mathcal{X}}
\newcommand{\cE}{\mathcal{E}}
\newcommand{\bbP}{\mathbb{P}}

We copy paste the proof from \cite{srinivas2012gaussian}
%@article{srinivas2012information,
%   title={Information-theoretic regret bounds for gaussian process optimization in the bandit setting},
%   author={Srinivas, Niranjan and Krause, Andreas and Kakade, Sham M and Seeger, Matthias W},
%   journal={IEEE transactions on information theory},
%   volume={58},
%   number={5},
%   pages={3250--3265},
%   year={2012},
%   publisher={IEEE}
% }

\begin{assumption}[GP bandit model]
Let $f:\cX\to\R$ be an unknown reward function. At each round $t=1,2,\dots$ an algorithm chooses $x_t\in\cX$
and observes
\begin{equation}\label{eq:obs-model}
y_t \;=\; f(x_t) + \varepsilon_t,
\end{equation}
where $\{\varepsilon_t\}_{t\ge 1}$ are conditionally $\sigma$-sub-Gaussian noise variables, i.e.,
$\E[\exp(\lambda \varepsilon_t)\mid \mathcal{F}_{t-1}] \le \exp(\tfrac{1}{2}\sigma^2\lambda^2)$
for all $\lambda\in\R$, where $\mathcal{F}_{t-1}$ is the sigma-field generated by past actions and observations.
Assume a Gaussian process prior on $f$ with mean function $0$ and covariance kernel $k$.
Denote by $\mu_{t-1}(x)$ and $\sigma_{t-1}(x)$ the GP posterior mean and standard deviation at $x\in\cX$
conditioned on $\{(x_s,y_s)\}_{s=1}^{t-1}$.
\end{assumption}

\paragraph{GP-UCB policy.}
Fix a nondecreasing sequence $\{\beta_t\}_{t\ge 1}$.
At round $t$, GP-UCB selects
\begin{equation}\label{eq:gp-ucb-policy}
x_t \in \argmax_{x\in\cX} \; \mu_{t-1}(x) + \sqrt{\beta_t}\,\sigma_{t-1}(x).
\end{equation}

\paragraph{Regret.}
Let $x^\star\in\argmax_{x\in\cX} f(x)$ be an optimal maximizer (assumed to exist).
Define the instantaneous and cumulative regret by
\begin{equation}\label{eq:regret-def}
r_t := f(x^\star)-f(x_t),\qquad
R_T := \sum_{t=1}^T r_t.
\end{equation}

\begin{lemma}[Uniform GP confidence bound]\label{lem:ucb-confidence}
Let $\delta\in(0,1)$ and let $\{\beta_t\}_{t\ge 1}$ be chosen such that, with probability at least $1-\delta$,
the event
\begin{equation}\label{eq:confidence-event}
\cE := \Big\{ \forall t\ge 1,\ \forall x\in\cX:\ |f(x)-\mu_{t-1}(x)| \le \sqrt{\beta_t}\,\sigma_{t-1}(x) \Big\}
\end{equation}
holds.
For example, if $\cX$ is finite, one may take
\begin{equation}\label{eq:beta-finite}
\beta_t \;=\; 2\log\!\Big(\frac{|\cX|\pi^2 t^2}{6\delta}\Big),
\end{equation}
which yields $\bbP(\cE)\ge 1-\delta$ by a Gaussian tail bound and a union bound over $x\in\cX$ and $t\ge 1$.
\end{lemma}

\begin{lemma}[Instantaneous regret is controlled by posterior uncertainty]\label{lem:instantaneous-regret}
On the event $\cE$ in \eqref{eq:confidence-event}, the GP-UCB action sequence \eqref{eq:gp-ucb-policy} satisfies
\begin{equation}\label{eq:rt-bound}
r_t \;\le\; 2\sqrt{\beta_t}\,\sigma_{t-1}(x_t)\qquad\text{for all }t\ge 1.
\end{equation}
\end{lemma}

\begin{proof}
Fix $t\ge 1$ and suppose $\cE$ holds.
By \eqref{eq:confidence-event},
\begin{equation}\label{eq:upper-fstar}
f(x^\star)\le \mu_{t-1}(x^\star)+\sqrt{\beta_t}\sigma_{t-1}(x^\star).
\end{equation}
Since $x_t$ maximizes the upper confidence bound in \eqref{eq:gp-ucb-policy},
\begin{equation}\label{eq:ucb-max}
\mu_{t-1}(x^\star)+\sqrt{\beta_t}\sigma_{t-1}(x^\star)
\le
\mu_{t-1}(x_t)+\sqrt{\beta_t}\sigma_{t-1}(x_t).
\end{equation}
Again by \eqref{eq:confidence-event},
\begin{equation}\label{eq:lower-ft}
f(x_t)\ge \mu_{t-1}(x_t)-\sqrt{\beta_t}\sigma_{t-1}(x_t).
\end{equation}
Combining \eqref{eq:upper-fstar}--\eqref{eq:lower-ft} yields
\[
r_t = f(x^\star)-f(x_t)
\le
\big(\mu_{t-1}(x_t)+\sqrt{\beta_t}\sigma_{t-1}(x_t)\big)
-
\big(\mu_{t-1}(x_t)-\sqrt{\beta_t}\sigma_{t-1}(x_t)\big)
=
2\sqrt{\beta_t}\sigma_{t-1}(x_t),
\]
which proves \eqref{eq:rt-bound}.
\end{proof}

\paragraph{Maximum information gain.}
For a set of query points $A=\{x_1,\dots,x_T\}\subset \cX$, let $f_A := (f(x))_{x\in A}$ and $y_A := (y(x))_{x\in A}$.
Define the \emph{maximum information gain} by
\begin{equation}\label{eq:gamma-def}
\gamma_T \;:=\; \max_{A\subset \cX,\ |A|=T} \I(y_A; f_A).
\end{equation}
In the Gaussian noise case, with kernel matrix $K_A \in \R^{T\times T}$ on $A$ and noise variance $\sigma^2$,
\begin{equation}\label{eq:mutual-info-gaussian}
\I(y_A;f_A) \;=\; \frac{1}{2}\log\det\!\big(I + \sigma^{-2}K_A\big).
\end{equation}

\begin{lemma}[Posterior variance sum is controlled by information gain]\label{lem:variance-sum}
Let $\{x_t\}_{t=1}^T$ be any sequence of query points and let $\sigma_{t-1}^2(x_t)$ be the GP posterior variance
at $x_t$ given data up to $t-1$.
Then there exists a constant $C_\sigma>0$ (depending only on the noise level) such that
\begin{equation}\label{eq:variance-sum}
\sum_{t=1}^T \sigma_{t-1}^2(x_t) \;\le\; C_\sigma\,\gamma_T.
\end{equation}
For instance, for homoscedastic Gaussian noise with variance $\sigma^2$ one may take
\begin{equation}\label{eq:Csigma}
C_\sigma \;=\; \frac{2}{\log(1+\sigma^{-2})},
\end{equation}
and \eqref{eq:variance-sum} holds (see, e.g., the GP-UCB analysis).
\end{lemma}

\begin{theorem}[GP-UCB regret bound]\label{thm:gp-ucb-regret}
Fix $\delta\in(0,1)$ and choose $\{\beta_t\}_{t\ge 1}$ such that the confidence event $\cE$ in
\eqref{eq:confidence-event} holds with probability at least $1-\delta$.
Assume $\beta_t$ is nondecreasing.
Then, with probability at least $1-\delta$, the cumulative regret of GP-UCB satisfies
\begin{equation}\label{eq:regret-main}
R_T \;\le\; 2\sqrt{C_\sigma\,T\,\beta_T\,\gamma_T}\qquad\text{for all }T\ge 1,
\end{equation}
where $\gamma_T$ is the maximum information gain in \eqref{eq:gamma-def} and $C_\sigma$ is as in
Lemma~\ref{lem:variance-sum}.
\end{theorem}

\begin{proof}
Work on the event $\cE$ (which holds w.p.\ $\ge 1-\delta$).
By Lemma~\ref{lem:instantaneous-regret} and monotonicity of $\beta_t$,
\begin{equation}\label{eq:rt-sum-step}
R_T = \sum_{t=1}^T r_t
\le
2\sum_{t=1}^T \sqrt{\beta_t}\,\sigma_{t-1}(x_t)
\le
2\sqrt{\beta_T}\sum_{t=1}^T \sigma_{t-1}(x_t).
\end{equation}
By Cauchy--Schwarz,
\begin{equation}\label{eq:cs}
\sum_{t=1}^T \sigma_{t-1}(x_t)
\le
\sqrt{T\sum_{t=1}^T \sigma_{t-1}^2(x_t)}.
\end{equation}
Combining \eqref{eq:rt-sum-step}--\eqref{eq:cs} and applying Lemma~\ref{lem:variance-sum} yields
\[
R_T
\le
2\sqrt{\beta_T}\sqrt{T\sum_{t=1}^T \sigma_{t-1}^2(x_t)}
\le
2\sqrt{\beta_T}\sqrt{T\cdot C_\sigma\,\gamma_T}
=
2\sqrt{C_\sigma\,T\,\beta_T\,\gamma_T},
\]
which proves \eqref{eq:regret-main}.
\end{proof}

\begin{remark}[Typical growth of $\gamma_T$]
For common kernels, $\gamma_T$ can be bounded as a function of $T$ and the input dimension $d$.
For example, for the squared-exponential (RBF) kernel on a compact subset of $\R^d$,
$\gamma_T = \tilde{\mathcal{O}}\big((\log T)^{d+1}\big)$, yielding sublinear regret
$R_T = \tilde{\mathcal{O}}\big(\sqrt{T}\,(\log T)^{(d+1)/2}\big)$ up to the growth of $\beta_T$.
\end{remark}

\subsubsection{Generalization to mixtures: loose max-k UCB}
 
\newcommand{\cF}{\mathcal{F}}

\begin{assumption}[Finite mixture of Gaussian processes]\label{ass:mogp}
Let $K\in\mathbb{N}$ and mixture weights $\pi_1,\dots,\pi_K$ satisfy $\pi_k>0$, $\sum_{k=1}^K \pi_k=1$.
A latent component index $z\in\{1,\dots,K\}$ is drawn as
\begin{equation}\label{eq:z-prior}
z \sim \mathrm{Categorical}(\pi_1,\dots,\pi_K).
\end{equation}
Conditioned on $z=k$, the unknown reward function $f:\cX\to\R$ is drawn from a GP prior
\begin{equation}\label{eq:gp-component}
f \mid (z=k) \sim \mathcal{GP}(0,\,k_k),
\end{equation}
with (known) covariance kernel $k_k$.
At each round $t\ge 1$, an algorithm chooses $x_t\in\cX$ and observes
\begin{equation}\label{eq:mogp-obs}
y_t = f(x_t) + \varepsilon_t,
\end{equation}
where $\{\varepsilon_t\}$ are conditionally $\sigma$-sub-Gaussian:
$\E[\exp(\lambda\varepsilon_t)\mid \cF_{t-1}] \le \exp(\tfrac12\sigma^2\lambda^2)$ for all $\lambda\in\R$,
and $\cF_{t-1}$ is the sigma-field generated by past $(x_s,y_s)_{s\le t-1}$.
\end{assumption}

\paragraph{Component posteriors.}
For each component $k\in\{1,\dots,K\}$, let $\mu_{t-1}^{(k)}(x)$ and $\sigma_{t-1}^{(k)}(x)$ denote the
GP posterior mean and standard deviation at $x\in\cX$ computed under the assumption $z=k$
using data $\{(x_s,y_s)\}_{s=1}^{t-1}$.
 
\paragraph{Regret.}
Let $x^\star\in\argmax_{x\in\cX} f(x)$ be an optimizer. Define
\begin{equation}\label{eq:mogp-regret}
r_t := f(x^\star)-f(x_t),\qquad R_T := \sum_{t=1}^T r_t.
\end{equation}
 
\paragraph{Robust MoGP-UCB.}
Fix nondecreasing sequences $\{\beta_t^{(k)}\}_{t\ge 1}$ for each component $k$.
Define the robust upper confidence bound
\begin{equation}\label{eq:robust-ucb}
U_t(x) \;:=\; \max_{k\in\{1,\dots,K\}}\Big\{ \mu_{t-1}^{(k)}(x) + \sqrt{\beta_t^{(k)}}\,\sigma_{t-1}^{(k)}(x)\Big\}.
\end{equation}
The MoGP-UCB action is
\begin{equation}\label{eq:mogp-ucb-policy}
x_t \in \argmax_{x\in\cX} U_t(x).
\end{equation}
 
\begin{lemma}[Uniform confidence tubes for all components]\label{lem:mogp-confidence}
Fix $\delta\in(0,1)$ and choose $\beta_t^{(k)}$ such that, with probability at least $1-\delta$,
the event
\begin{equation}\label{eq:mogp-E}
\mathcal{E} := \Big\{\forall t\ge 1,\ \forall x\in\cX,\ \forall k\in\{1,\dots,K\}:\ 
|f(x)-\mu_{t-1}^{(k)}(x)| \le \sqrt{\beta_t^{(k)}}\,\sigma_{t-1}^{(k)}(x)\Big\}
\end{equation}
holds.
For finite $\cX$ one convenient choice is
\begin{equation}\label{eq:beta-mogp-finite}
\beta_t^{(k)} \;=\; 2\log\!\Big(\frac{K\,|\cX|\,\pi^2 t^2}{6\delta}\Big),
\end{equation}
which yields $\bbP(\mathcal{E})\ge 1-\delta$ by a Gaussian tail bound and a union bound over $(t,x,k)$.
\end{lemma}
  
\begin{lemma}[Instantaneous regret under robust MoGP-UCB]\label{lem:mogp-instantaneous}
On the event $\mathcal{E}$ in \eqref{eq:mogp-E}, the robust MoGP-UCB policy \eqref{eq:mogp-ucb-policy} satisfies
\begin{equation}\label{eq:mogp-rt}
r_t \;\le\; 2\sqrt{\beta_t^{(z)}}\,\sigma_{t-1}^{(z)}(x_t)\qquad \text{for all }t\ge 1.
\end{equation}
\end{lemma}

\begin{proof}
Assume $\mathcal{E}$ holds and fix $t\ge 1$.
Using \eqref{eq:mogp-E} with the \emph{true} component $z$,
\begin{equation}\label{eq:mogp-upper-fstar}
f(x^\star)\le \mu_{t-1}^{(z)}(x^\star)+\sqrt{\beta_t^{(z)}}\,\sigma_{t-1}^{(z)}(x^\star).
\end{equation}
By definition of $U_t$ in \eqref{eq:robust-ucb},
\begin{equation}\label{eq:mogp-ucb-dominates}
\mu_{t-1}^{(z)}(x^\star)+\sqrt{\beta_t^{(z)}}\,\sigma_{t-1}^{(z)}(x^\star)
\le U_t(x^\star).
\end{equation}
Since $x_t$ maximizes $U_t(\cdot)$,
\begin{equation}\label{eq:mogp-max}
U_t(x^\star)\le U_t(x_t).
\end{equation}
Also, $U_t(x_t)\ge \mu_{t-1}^{(z)}(x_t)+\sqrt{\beta_t^{(z)}}\,\sigma_{t-1}^{(z)}(x_t)$ by the max over $k$.
Finally, again from \eqref{eq:mogp-E} with component $z$,
\begin{equation}\label{eq:mogp-lower-ft}
f(x_t)\ge \mu_{t-1}^{(z)}(x_t)-\sqrt{\beta_t^{(z)}}\,\sigma_{t-1}^{(z)}(x_t).
\end{equation}
Combining \eqref{eq:mogp-upper-fstar}--\eqref{eq:mogp-lower-ft} yields
\[
r_t = f(x^\star)-f(x_t)
\le
2\sqrt{\beta_t^{(z)}}\,\sigma_{t-1}^{(z)}(x_t),
\]
which proves \eqref{eq:mogp-rt}.
\end{proof}
 
\paragraph{Information gain for component $k$.}
For a set $A=\{x_1,\dots,x_T\}\subset\cX$, define
\begin{equation}\label{eq:gamma-k}
\gamma_T^{(k)} := \max_{A\subset\cX,\ |A|=T}\I\big(y_A;\ f_A \,\big|\, z=k\big).
\end{equation}
In the homoscedastic Gaussian noise case, with kernel matrix $K_A^{(k)}$,
\begin{equation}\label{eq:gamma-k-gaussian}
\I\big(y_A;\ f_A \,\big|\, z=k\big) = \frac12\log\det\!\big(I+\sigma^{-2}K_A^{(k)}\big).
\end{equation}

\begin{lemma}[Variance sum bound (component-wise)]\label{lem:mogp-variance-sum}
There exists a constant $C_\sigma>0$ (depending only on the noise level) such that for any query sequence
$\{x_t\}_{t=1}^T$ and any component $k$,
\begin{equation}\label{eq:mogp-variance-sum}
\sum_{t=1}^T \big(\sigma_{t-1}^{(k)}(x_t)\big)^2 \;\le\; C_\sigma\,\gamma_T^{(k)}.
\end{equation}
For homoscedastic Gaussian noise variance $\sigma^2$, one admissible choice is
$C_\sigma = 2/\log(1+\sigma^{-2})$.
\end{lemma}
 
\begin{theorem}[MoGP-UCB regret bound]\label{thm:mogp-regret}
Fix $\delta\in(0,1)$ and choose $\{\beta_t^{(k)}\}$ so that the uniform event $\mathcal{E}$ in \eqref{eq:mogp-E}
holds with probability at least $1-\delta$ (e.g.\ \eqref{eq:beta-mogp-finite} for finite $\cX$).
Assume each $\beta_t^{(k)}$ is nondecreasing in $t$.
Then, with probability at least $1-\delta$, the cumulative regret of robust MoGP-UCB satisfies
\begin{equation}\label{eq:mogp-main-regret}
R_T \;\le\; 2\sqrt{C_\sigma\,T\,\beta_T^{(z)}\,\gamma_T^{(z)}}\qquad\text{for all }T\ge 1,
\end{equation}
where $z$ is the (unknown) latent component generating $f$ and $\gamma_T^{(z)}$ is defined in \eqref{eq:gamma-k}.
In particular, a component-uniform (worst-case) bound is
\begin{equation}\label{eq:mogp-worstcase}
R_T \;\le\; 2\sqrt{C_\sigma\,T\,\Big(\max_{k}\beta_T^{(k)}\Big)\,\Big(\max_{k}\gamma_T^{(k)}\Big)}.
\end{equation}
\end{theorem}

\begin{proof}
Work on the event $\mathcal{E}$.
By Lemma~\ref{lem:mogp-instantaneous} and monotonicity of $\beta_t^{(z)}$,
\begin{align}
R_T
= \sum_{t=1}^T r_t
&\le 2\sum_{t=1}^T \sqrt{\beta_t^{(z)}}\,\sigma_{t-1}^{(z)}(x_t)
\le 2\sqrt{\beta_T^{(z)}}\sum_{t=1}^T \sigma_{t-1}^{(z)}(x_t).
\end{align}
Cauchy--Schwarz gives
\[
\sum_{t=1}^T \sigma_{t-1}^{(z)}(x_t)
\le \sqrt{T\sum_{t=1}^T \big(\sigma_{t-1}^{(z)}(x_t)\big)^2}.
\]
Apply Lemma~\ref{lem:mogp-variance-sum} with $k=z$ to obtain
\[
R_T \le 2\sqrt{\beta_T^{(z)}}\sqrt{T\cdot C_\sigma\,\gamma_T^{(z)}}
= 2\sqrt{C_\sigma\,T\,\beta_T^{(z)}\,\gamma_T^{(z)}}.
\]
The worst-case bound \eqref{eq:mogp-worstcase} follows immediately.
\end{proof}

\begin{remark}[Bayesian regret over the mixture]
Taking expectation w.r.t.\ $z\sim\mathrm{Categorical}(\pi)$,
\[
\E[R_T] \le 2\sqrt{C_\sigma\,T}\ \sum_{k=1}^K \pi_k \sqrt{\beta_T^{(k)}\,\gamma_T^{(k)}}
\le 2\sqrt{C_\sigma\,T}\ \sqrt{\sum_{k=1}^K \pi_k \beta_T^{(k)}\,\gamma_T^{(k)}},
\]
where the last inequality is Jensen (concavity of $\sqrt{\cdot}$).
\end{remark}

\subsection{Generalization to mixtures: Moment-matched UCB}

\begin{assumption}[Mixture-of-GPs bandit model]\label{ass:mogp-mm}
Let $K\in\mathbb{N}$ and mixture weights $\pi_1,\dots,\pi_K$ satisfy $\pi_k>0$, $\sum_{k=1}^K \pi_k=1$.
A latent component index $z\in\{1,\dots,K\}$ is drawn as
\begin{equation}\label{eq:mm-z-prior}
z \sim \mathrm{Categorical}(\pi_1,\dots,\pi_K).
\end{equation}
Conditioned on $z=k$, the unknown reward function $f:\cX\to\R$ is drawn from a GP prior
\begin{equation}\label{eq:mm-gp-component}
f \mid (z=k) \sim \mathcal{GP}(0,\,k_k),
\end{equation}
with known kernel $k_k$. At each round $t\ge 1$, an algorithm chooses $x_t\in\cX$ and observes
\begin{equation}\label{eq:mm-obs}
y_t = f(x_t) + \varepsilon_t,
\end{equation}
where $\{\varepsilon_t\}$ are conditionally $\sigma$-sub-Gaussian:
$\E[\exp(\lambda\varepsilon_t)\mid \cF_{t-1}] \le \exp(\tfrac12\sigma^2\lambda^2)$ for all $\lambda\in\R$,
with $\cF_{t-1}$ generated by past $(x_s,y_s)_{s\le t-1}$.
\end{assumption}

\paragraph{Component posteriors.}
For each $k\in\{1,\dots,K\}$, let $\mu_{t-1}^{(k)}(x)$ and $\sigma_{t-1}^{(k)}(x)$ denote the GP posterior mean
and standard deviation at $x\in\cX$ computed under the conditional model $z=k$ using data
$\mathcal{D}_{t-1} := \{(x_s,y_s)\}_{s=1}^{t-1}$.
 
\paragraph{Posterior responsibilities.}
Let $w_{t-1}^{(k)} := \bbP(z=k \mid \mathcal{D}_{t-1})$.
By Bayes' rule,
\begin{equation}\label{eq:mm-resp}
w_{t-1}^{(k)}
=
\frac{\pi_k\,p(\mathcal{D}_{t-1}\mid z=k)}{\sum_{j=1}^K \pi_j\,p(\mathcal{D}_{t-1}\mid z=j)}.
\end{equation}
In the Gaussian noise case, $p(\mathcal{D}_{t-1}\mid z=k)$ is the standard GP marginal likelihood
(with kernel $k_k$ and noise variance $\sigma^2$).
 
\paragraph{Moment-matched predictive mean and variance.}
Let $\mathcal{D}_{t-1}$ be fixed. The exact predictive distribution of $f(x)$ under the mixture posterior is
\begin{equation}\label{eq:mm-mixture-posterior}
p\big(f(x)\mid \mathcal{D}_{t-1}\big)
=
\sum_{k=1}^K w_{t-1}^{(k)}\,
p\big(f(x)\mid \mathcal{D}_{t-1}, z=k\big),
\end{equation}
where $p(f(x)\mid \mathcal{D}_{t-1}, z=k)$ is Gaussian with mean $\mu_{t-1}^{(k)}(x)$ and variance
$(\sigma_{t-1}^{(k)}(x))^2$.

Define the moment-matched mean and variance by, see result in the main paper.
\begin{equation}\label{eq:mm-def-moments}
\mu_{t-1}^{\mathrm{mix}}(x) := \E\big[f(x)\mid \mathcal{D}_{t-1}\big],\qquad
\big(\sigma_{t-1}^{\mathrm{mix}}(x)\big)^2 := \Var\big(f(x)\mid \mathcal{D}_{t-1}\big).
\end{equation}

\paragraph{MM-MoGP-UCB policy.}
Fix a nondecreasing exploration sequence $\{\beta_t\}_{t\ge 1}$ and define
\begin{equation}\label{eq:mm-ucb}
U_t^{\mathrm{mix}}(x) := \mu_{t-1}^{\mathrm{mix}}(x) + \sqrt{\beta_t}\,\sigma_{t-1}^{\mathrm{mix}}(x).
\end{equation}
The moment-matched UCB action is
\begin{equation}\label{eq:mm-policy}
x_t \in \argmax_{x\in\cX} U_t^{\mathrm{mix}}(x).
\end{equation}

\paragraph{Regret.}
Let $x^\star\in\argmax_{x\in\cX} f(x)$ and define
\begin{equation}\label{eq:mm-regret}
r_t := f(x^\star)-f(x_t),\qquad R_T := \sum_{t=1}^T r_t.
\end{equation}
 
\begin{assumption}[Component-wise confidence tubes]\label{ass:mm-comp-tubes}
Fix $\delta\in(0,1)$ and choose (component-wise) $\{\beta_t^{(k)}\}_{t\ge 1}$ such that with probability at least
$1-\delta$,
\begin{equation}\label{eq:mm-comp-event}
\mathcal{E}_{\mathrm{comp}}
:=
\Big\{ \forall t\ge 1,\ \forall x\in\cX,\ \forall k\in\{1,\dots,K\}:\ 
|f(x)-\mu_{t-1}^{(k)}(x)| \le \sqrt{\beta_t^{(k)}}\,\sigma_{t-1}^{(k)}(x)\Big\}
\end{equation}
holds (e.g.\ for finite $\cX$ via a union bound over $(t,x,k)$).
\end{assumption}

\begin{assumption}[Lower bound on responsibility of the true component]\label{ass:mm-weight-lb}
There exists $\underline{w}\in(0,1]$ such that, for all $t\ge 1$,
\begin{equation}\label{eq:mm-weight-lb}
w_{t-1}^{(z)} = \bbP(z\mid \mathcal{D}_{t-1}) \ge \underline{w}.
\end{equation}
(For example, this can be enforced by truncating responsibilities away from $0$ in implementation,
or it may follow from additional identifiability/likelihood-ratio conditions.)
\end{assumption}

\begin{lemma}[Two deterministic inequalities linking $(\mu^{(z)},\sigma^{(z)})$ to $(\mu^{\mathrm{mix}},\sigma^{\mathrm{mix}})$]
\label{lem:mm-det-ineq}
Fix $t\ge 1$ and $x\in\cX$. Let $w:=w_{t-1}^{(z)}$.
Then
\begin{align}
\big(\sigma_{t-1}^{\mathrm{mix}}(x)\big)^2
&\ge
w\,\big(\sigma_{t-1}^{(z)}(x)\big)^2,
\label{eq:mm-sig-dom}\\
\big(\sigma_{t-1}^{\mathrm{mix}}(x)\big)^2
&\ge
w\,\big(\mu_{t-1}^{(z)}(x)-\mu_{t-1}^{\mathrm{mix}}(x)\big)^2.
\label{eq:mm-mean-gap-dom}
\end{align}
Consequently,
\begin{equation}\label{eq:mm-gap-bounds}
\sigma_{t-1}^{(z)}(x) \le \frac{1}{\sqrt{w}}\sigma_{t-1}^{\mathrm{mix}}(x),\qquad
\big|\mu_{t-1}^{(z)}(x)-\mu_{t-1}^{\mathrm{mix}}(x)\big|\le \frac{1}{\sqrt{w}}\sigma_{t-1}^{\mathrm{mix}}(x).
\end{equation}
\end{lemma}

\begin{proof}
From \eqref{eq:mm-var}, since all terms are nonnegative and $w_{t-1}^{(z)}=w$,
\[
\big(\sigma_{t-1}^{\mathrm{mix}}(x)\big)^2
=
\sum_{k=1}^K w_{t-1}^{(k)}\Big((\sigma_{t-1}^{(k)}(x))^2 + (\mu_{t-1}^{(k)}(x)-\mu_{t-1}^{\mathrm{mix}}(x))^2\Big)
\ge
w\,(\sigma_{t-1}^{(z)}(x))^2,
\]
proving \eqref{eq:mm-sig-dom}. Dropping the within-component variance terms instead yields
\[
\big(\sigma_{t-1}^{\mathrm{mix}}(x)\big)^2 \ge w\,(\mu_{t-1}^{(z)}(x)-\mu_{t-1}^{\mathrm{mix}}(x))^2,
\]
proving \eqref{eq:mm-mean-gap-dom}. Taking square roots gives \eqref{eq:mm-gap-bounds}.
\end{proof}

\begin{lemma}[Sufficient confidence tube for the moment-matched moments]\label{lem:mm-mix-confidence}
Assume $\mathcal{E}_{\mathrm{comp}}$ holds. Then for all $t\ge 1$ and $x\in\cX$,
\begin{equation}\label{eq:mm-mix-tube-pre}
|f(x)-\mu_{t-1}^{\mathrm{mix}}(x)|
\le
\left(\frac{\sqrt{\beta_t^{(z)}}+1}{\sqrt{w_{t-1}^{(z)}}}\right)\sigma_{t-1}^{\mathrm{mix}}(x).
\end{equation}
Under Assumption~\ref{ass:mm-weight-lb}, i.e.\ $w_{t-1}^{(z)}\ge \underline{w}$, the uniform tube
\begin{equation}\label{eq:mm-mix-tube}
|f(x)-\mu_{t-1}^{\mathrm{mix}}(x)| \le \sqrt{\beta_t}\,\sigma_{t-1}^{\mathrm{mix}}(x)
\qquad\text{for all }t\ge 1,\ x\in\cX
\end{equation}
holds with
\begin{equation}\label{eq:mm-beta-choice}
\beta_t := \frac{\big(\sqrt{\beta_t^{\max}}+1\big)^2}{\underline{w}},
\qquad \beta_t^{\max} := \max_{k\in\{1,\dots,K\}}\beta_t^{(k)}.
\end{equation}
\end{lemma}

\begin{proof}
Fix $t,x$ and write $w:=w_{t-1}^{(z)}$.
By the triangle inequality,
\begin{equation}\label{eq:mm-tri}
|f(x)-\mu_{t-1}^{\mathrm{mix}}(x)|
\le
|f(x)-\mu_{t-1}^{(z)}(x)|
+
|\mu_{t-1}^{(z)}(x)-\mu_{t-1}^{\mathrm{mix}}(x)|.
\end{equation}
On $\mathcal{E}_{\mathrm{comp}}$, the first term is bounded by $\sqrt{\beta_t^{(z)}}\,\sigma_{t-1}^{(z)}(x)$.
Apply \eqref{eq:mm-gap-bounds} to both terms:
\[
|f(x)-\mu_{t-1}^{\mathrm{mix}}(x)|
\le
\sqrt{\beta_t^{(z)}}\frac{1}{\sqrt{w}}\sigma_{t-1}^{\mathrm{mix}}(x)
+
\frac{1}{\sqrt{w}}\sigma_{t-1}^{\mathrm{mix}}(x)
=
\left(\frac{\sqrt{\beta_t^{(z)}}+1}{\sqrt{w}}\right)\sigma_{t-1}^{\mathrm{mix}}(x),
\]
proving \eqref{eq:mm-mix-tube-pre}. Under $w\ge \underline{w}$ and $\beta_t^{(z)}\le \beta_t^{\max}$,
\[
\left(\frac{\sqrt{\beta_t^{(z)}}+1}{\sqrt{w}}\right)^2
\le
\frac{(\sqrt{\beta_t^{\max}}+1)^2}{\underline{w}}=\beta_t,
\]
which yields \eqref{eq:mm-mix-tube}.
\end{proof}
 
\begin{lemma}[Instantaneous regret for MM-MoGP-UCB]\label{lem:mm-inst-regret}
Assume the moment-matched tube \eqref{eq:mm-mix-tube} holds (e.g.\ by Lemma~\ref{lem:mm-mix-confidence}).
Then the MM-MoGP-UCB policy \eqref{eq:mm-policy} satisfies
\begin{equation}\label{eq:mm-rt}
r_t \le 2\sqrt{\beta_t}\,\sigma_{t-1}^{\mathrm{mix}}(x_t)\qquad\text{for all }t\ge 1.
\end{equation}
\end{lemma}

\begin{proof}
Identical to the standard GP-UCB proof: on \eqref{eq:mm-mix-tube},
\[
f(x^\star)\le \mu_{t-1}^{\mathrm{mix}}(x^\star)+\sqrt{\beta_t}\sigma_{t-1}^{\mathrm{mix}}(x^\star)
\le
\mu_{t-1}^{\mathrm{mix}}(x_t)+\sqrt{\beta_t}\sigma_{t-1}^{\mathrm{mix}}(x_t),
\]
and also $f(x_t)\ge \mu_{t-1}^{\mathrm{mix}}(x_t)-\sqrt{\beta_t}\sigma_{t-1}^{\mathrm{mix}}(x_t)$,
which together imply \eqref{eq:mm-rt}.
\end{proof}
 
\paragraph{A variance-sum control for moment-matched uncertainty.}
The standard GP-UCB regret proof closes by bounding $\sum_{t\le T}\sigma_{t-1}^2(x_t)$ via information gain.
For the moment-matched mixture variance $\big(\sigma_{t-1}^{\mathrm{mix}}(\cdot)\big)^2$, the posterior is
not Gaussian; thus one typically assumes or proves an analogue of the variance-sum lemma.

\begin{assumption}[Variance-sum bound for moment-matched uncertainty]\label{ass:mm-varsum}
There exist a functional $\gamma_T^{\mathrm{mix}}$ (interpretable as a complexity / information-gain term for the
moment-matched model) and a constant $C_\sigma>0$ such that for any query sequence $\{x_t\}_{t=1}^T$,
\begin{equation}\label{eq:mm-varsum}
\sum_{t=1}^T \big(\sigma_{t-1}^{\mathrm{mix}}(x_t)\big)^2 \le C_\sigma\,\gamma_T^{\mathrm{mix}}.
\end{equation}
\end{assumption}

\begin{theorem}[MM-MoGP-UCB regret bound (template)]\label{thm:mm-regret}
Fix $\delta\in(0,1)$ and suppose Assumptions~\ref{ass:mm-comp-tubes} and \ref{ass:mm-weight-lb} hold,
so that the moment-matched tube \eqref{eq:mm-mix-tube} holds with probability at least $1-\delta$
(e.g.\ via Lemma~\ref{lem:mm-mix-confidence} and a union bound for $\mathcal{E}_{\mathrm{comp}}$).
Assume $\beta_t$ is nondecreasing and Assumption~\ref{ass:mm-varsum} holds.
Then with probability at least $1-\delta$, the cumulative regret of MM-MoGP-UCB satisfies
\begin{equation}\label{eq:mm-main-regret}
R_T \le 2\sqrt{C_\sigma\,T\,\beta_T\,\gamma_T^{\mathrm{mix}}}\qquad \text{for all }T\ge 1.
\end{equation}
\end{theorem}

\begin{proof}
On the tube \eqref{eq:mm-mix-tube}, Lemma~\ref{lem:mm-inst-regret} yields
\[
R_T \le 2\sum_{t=1}^T \sqrt{\beta_t}\,\sigma_{t-1}^{\mathrm{mix}}(x_t)
\le 2\sqrt{\beta_T}\sum_{t=1}^T \sigma_{t-1}^{\mathrm{mix}}(x_t).
\]
Cauchy--Schwarz gives $\sum_{t=1}^T \sigma_{t-1}^{\mathrm{mix}}(x_t)\le
\sqrt{T\sum_{t=1}^T(\sigma_{t-1}^{\mathrm{mix}}(x_t))^2}$, and Assumption~\ref{ass:mm-varsum} closes the bound.
\end{proof}
