# Supplementary material for: Regime-Adaptive Bayesian Optimization via Dirichlet Process Mixtures of Gaussian Processes
Source: arXiv:2601.20043 source file (2026-07-28)
Supplement: Supplementary file 2 [file suppl_sascha.tex]

\section{MES}

\subsection{Max-value Entropy Search (MES)}

We further extend the DPMM-GP to entropy-based search. Max-value Entropy Search (MES) seeks to maximize the mutual information between the candidate observation $y$ at $\mathbf{x}$ and the global maximum value $y^* = \max_{\mathbf{x}' \in \mathcal{X}} f(\mathbf{x}')$. The acquisition function is defined as:
\begin{equation}
	\alpha_{\text{MES}}(\mathbf{x}) = H(y \mid \mathbf{x}) - \mathbb{E}_{y^*} \left[ H(y \mid \mathbf{x}, y < y^*) \right].
\end{equation}

For the DPMM-GP, the first term $H(y \mid \mathbf{x})$ is the entropy of the predictive mixture derived in Theorem \ref{thm:predictive}. While the entropy of a Gaussian mixture has no closed form, we approximate it via the entropy of a single Gaussian with moment-matched variance $\sigma^2_{\text{mix}}(\mathbf{x})$:
\begin{equation}
	H(y \mid \mathbf{x}) \approx \frac{1}{2} \log(2\pi e \sigma^2_{\text{mix}}(\mathbf{x})).
\end{equation}

For the second term, we estimate the expectation over $y^*$ via Monte Carlo sampling. We sample $y^*_s \sim p(y^*)$ by first sampling a regime $k \sim \boldsymbol{\pi}$ and then sampling the maximum of that GP component (e.g., via Gumbel approximation). Given a sample $y^*_s$, the conditional entropy is computed using the truncated Gaussian approximation for each component weighted by $w_k(\mathbf{x})$:
\begin{equation}
	\mathbb{E}_{y^*} [H(\dots)] \approx \frac{1}{S} \sum_{s=1}^S \sum_{k=1}^K w_k(\mathbf{x}) \left[ \frac{\gamma_{k,s} \phi(\gamma_{k,s})}{2\Phi(\gamma_{k,s})} - \ln \Phi(\gamma_{k,s}) \right],
\end{equation}
where $\gamma_{k,s} = (y^*_s - \mu_{*,k}(\mathbf{x})) / \sigma_{*,k}(\mathbf{x})$. This formulation directs sampling toward regions that maximally reduce uncertainty about the global maximum across all latent regimes.

\newpage

\section{Complete Optimization Loop of \ours}

\ours integrates the DPMM-GP surrogate with a sequential acquisition strategy. The complete procedure is outlined in Algorithm \ref{alg:bo_loop} and proceeds through four distinct phases at each iteration $t$:

\begin{enumerate}
	\item \textbf{Initialization:} We initialize the procedure with a small seed dataset $\mathcal{D}_0$ generated via Latin Hypercube Sampling (LHS) to ensuring a space-filling coverage of the domain $\mathcal{X}$ before the model guides the search.
	
	\item \textbf{Inference with Warm Starts:} To reduce the computational burden of MCMC, we employ a \textit{warm start} strategy. Instead of re-initializing the sampler from scratch, we initialize the Gibbs sampler (Algorithm \ref{alg:gibbs}) using the assignments $\mathbf{z}^{(t-1)}$ and hyperparameters $\Theta^{(t-1)}$ from the previous iteration. This significantly reduces the burn-in period required to reach the stationary distribution.
	
	\item \textbf{Acquisition Optimization:} We maximize the mixture Expected Improvement $\alpha_{\text{EI}}(\mathbf{x})$. Since the acquisition landscape is inherently multimodal (inheriting local optima from multiple regime-specific GPs), we optimize it using a multi-start L-BFGS-B approach. The optimizer is initialized with a hybrid set of candidates $\mathcal{S}_{init}$ comprising: (1) uniform random samples, (2) centroids of currently active regimes, and (3) local perturbations of the current best solution $\mathbf{x}^*$.
	
	\item \textbf{Feedback and Maintenance:} After evaluating the selected candidate $\mathbf{x}_{new}$, we augment the dataset and perform a maintenance step. We prune any ``dead'' regimes (empty clusters or weights $\pi_k < \epsilon$) to maintain a compact model representation and prevent unnecessary computation in subsequent matrix inversions.
\end{enumerate}

\begin{algorithm}[h]
	\caption{DPMM-GP Bayesian Optimization Loop}
	\label{alg:bo_loop}
	\begin{algorithmic}[1]
		\STATE {\bfseries Input:} Search space $\mathcal{X}$, budget $T_{\text{max}}$, initial size $n_{\text{init}}$
		\STATE {\bfseries Parameters:} MCMC samples $S$, restarts $R$, prune threshold $\epsilon$
		\STATE {\bfseries Output:} Best solution $\mathbf{x}^*$
		
		\STATE \textit{// Phase 1: Initialization}
		\STATE $\mathcal{D}_0 \leftarrow$ LatinHypercubeSampling($\mathcal{X}, n_{\text{init}}$)
		\STATE Initialize $\Theta^{(0)}$ and $\mathbf{z}^{(0)}$ randomly
		\STATE $\mathbf{x}^* \leftarrow \text{argmax}_{(\mathbf{x},y) \in \mathcal{D}_0} y$
		
		\FOR{$t = 1$ {\bfseries to} $T_{\text{max}}$}
		\STATE \textit{// Phase 2: Inference (Warm Start)}
		\STATE Run Collapsed Gibbs (Alg. \ref{alg:gibbs}) for $S$ steps initialized with $(\Theta^{(t-1)}, \mathbf{z}^{(t-1)})$
		\STATE Collect posterior samples $\{\Theta^{(s)}, \mathbf{z}^{(s)}\}_{s=1}^S$
		\STATE Compute mixture moments $\mu_{\text{mix}}(\mathbf{x}), \sigma_{\text{mix}}(\mathbf{x})$ and weights $w_k(\mathbf{x})$ (Thm. \ref{thm:mixture_stats})
		
		\STATE \textit{// Phase 3: Acquisition Optimization}
		\STATE Define $\alpha_{\text{EI}}(\mathbf{x})$ per Eq. \eqref{eq:ei_dpmm}
		\STATE Generate start points $\mathcal{S}_{init} \leftarrow \{ \text{Uniform}(\mathcal{X}) \} \cup \{ \text{Centroids}(\mathbf{z}) \} \cup \{ \mathbf{x}^* + \delta \}$
		\STATE $\mathbf{x}_{new} \leftarrow \text{argmax}_{\mathbf{x} \in \mathcal{S}_{init}} \text{L-BFGS-B}(\alpha_{\text{EI}}(\mathbf{x}))$
		
		\STATE \textit{// Phase 4: Evaluation \& Update}
		\STATE $y_{new} \leftarrow f(\mathbf{x}_{new}) + \varepsilon$
		\STATE $\mathcal{D}_t \leftarrow \mathcal{D}_{t-1} \cup \{(\mathbf{x}_{new}, y_{new})\}$
		\IF{$y_{new} > f(\mathbf{x}^*)$}
		\STATE $\mathbf{x}^* \leftarrow \mathbf{x}_{new}$
		\ENDIF
		
		\STATE \textit{// Phase 5: Maintenance}
		\STATE Update $(\Theta^{(t)}, \mathbf{z}^{(t)})$ using the last MCMC sample
		\STATE Prune regimes where $\sum_i \mathbb{I}(z_i = k) < 1$ or $\pi_k < \epsilon$
		\ENDFOR
	\end{algorithmic}
\end{algorithm}

\newpage
